# Supplementary material for: Accessible precisions for estimating two conjugate parameters using Gaussian probes
Source: arXiv:2003.07095 ancillary file (2020-03-19)
Supplement: Supplementary file 1 [file qrs_supplementary.pdf]

# Supplementary material: Accessible precisions for estimating two conjugate parameters using Gaussian probes

Syed M. Assad,[1,2,3,*] Jiamin Li,[1] Yuhong Liu,[1] Ningbo Zhao,[1]
Wen Zhao,[1] Ping Koy Lam,[3] Z. Y. Ou,[1,4,†] and Xiaoying Li[1,‡]

[1] *College of Precision Instrument and Opto-Electronics Engineering, Key Laboratory of Opto-Electronics Information Technology, Ministry of Education, Tianjin University, Tianjin 300072, China.*
[2] *School of Physical and Mathematical Sciences, Nanyang Technological University, Singapore 639673.*
[3] *Centre for Quantum Computation and Communication Technology, Department of Quantum Science, Research School of Physics and Engineering, Australian National University, Canberra ACT 2601, Australia.*
[4] *Department of Physics, Indiana University-Purdue University Indianapolis, Indianapolis, IN 46202, USA.*

(Dated: March 16, 2020)

In this supplementary material, we introduce some preliminaries and notations in section I that will be used to derive the results in the main text. Section II details the steps leading to the results for a single mode probe and section III for a two-mode probe. In Section IV, we consider the effect of channel noise and lossy detectors on the achievable precision with a two-mode probe.

## I. PRELIMINARIES AND NOTATIONS

We define the following operators:

| | |
|---|---|
| $X = a + a^\dagger$ | Amplitude quadrature operator |
| $Y = \mathrm{i}\left(a^\dagger - a\right)$ | Phase quadrature operator |
| $\Phi(\phi) = \exp(\mathrm{i}\phi\, a^\dagger a)$ | Phase shift operator |
| $D(\alpha) = \exp(\alpha a^\dagger - \bar{\alpha} a)$ | Displacement operator |
| $D(\theta_x, \theta_y) = \exp\left(\frac{i\theta_y}{2}X - \frac{i\theta_x}{2}Y\right)$ | Displacement operator |
| $S(r) = \exp\left(\frac{r}{2}(a^2 - {a^\dagger}^2)\right)$ | Squeezing operator |
| $B(\vartheta) = \exp\left(\vartheta(a_1^\dagger a_2 - a_1 a_2^\dagger)\right)$ | Beam-mixing operator |

where $\theta_x = 2\mathrm{Re}\alpha$ and $\theta_y = 2\mathrm{Im}\alpha$. The beam-splitter transmission will be $t = \cos^2\vartheta$.

### A. Relations for single-mode operations

Some elementary relations that will come in useful are listed below.

$$\Phi^\dagger(\phi)D(\theta_x,\theta_y)\Phi(\phi) = D(\theta_x\cos\phi + \theta_y\sin\phi, \theta_y\cos\phi - \theta_x\sin\phi) \tag{1}$$

$$\frac{\partial}{\partial\theta_x}\left(\Phi^\dagger(\phi)D(\theta_x,\theta_y)\Phi(\phi)\right)\Big|_{\theta=0} = -\frac{\mathrm{i}}{2}X\sin\phi - \frac{\mathrm{i}}{2}Y\cos\phi \tag{2}$$

$$\frac{\partial}{\partial\theta_y}\left(\Phi^\dagger(\phi)D(\theta_x,\theta_y)\Phi(\phi)\right)\Big|_{\theta=0} = \frac{\mathrm{i}}{2}X\cos\phi - \frac{\mathrm{i}}{2}Y\sin\phi \tag{3}$$

$$\tag{4}$$

* cqtsma@gmail.com
† zou@iupui.edu
‡ xiaoyingli@tju.edu.cn

The squeezed state $|S(r)\rangle = S(r)|0\rangle$ has the following expectation values

$$\langle S(r)|X|S(r)\rangle = 0\ , \tag{5}$$
$$\langle S(r)|Y|S(r)\rangle = 0\ , \tag{6}$$
$$\left\langle S(r)\middle|X^2\middle|S(r)\right\rangle = \exp(-2r)\ , \tag{7}$$
$$\left\langle S(r)\middle|Y^2\middle|S(r)\right\rangle = \exp(2r)\ , \tag{8}$$
$$\langle S(r)|XY|S(r)\rangle = \mathrm{i}\ . \tag{9}$$

### B. Relations for two-mode operations

Some elementary relations that will come in useful are listed below.

$$\Phi^\dagger(\phi_1,\phi_2)B_{12}^\dagger(t)D_2(\theta_x,\theta_y)B_{12}(t)\Phi(\phi_1,\phi_2) \tag{10}$$
$$=\Phi^\dagger(\phi_1,\phi_2)B_{12}^\dagger(t)D_1(-\sqrt{1-t}\theta_x,-\sqrt{1-t}\theta_y)D_2(\sqrt{t}\theta_x,\sqrt{t}\theta_y)\Phi(\phi_1,\phi_2) \tag{11}$$
$$=D_1(-\sqrt{1-t}\theta_x\cos\phi_1-\sqrt{1-t}\theta_y\sin\phi_1,-\sqrt{1-t}\theta_y\cos\phi_1+\sqrt{1-t}\theta_x\sin\phi_1) \tag{12}$$
$$\otimes D_2(\sqrt{t}\theta_x\cos\phi_2+\sqrt{t}\theta_y\sin\phi_2,\sqrt{t}\theta_y\cos\phi_2-\sqrt{t}\theta_x\sin\phi_2)\ . \tag{13}$$

$$\frac{\partial}{\partial\theta_x}\Big(\Phi^\dagger(\phi_1,\phi_2)B_{12}^\dagger(t)D_2(\theta_x,\theta_y)B_{12}(t)\Phi(\phi_1,\phi_2)\Big)\Big|_{\theta=0} \tag{14}$$
$$=\left(\frac{\mathrm{i}}{2}\sqrt{1-t}X_1\sin\phi_1+\frac{\mathrm{i}}{2}\sqrt{1-t}Y_1\cos\phi_1\right)+\left(-\frac{\mathrm{i}}{2}\sqrt{t}X_2\sin\phi_2-\frac{\mathrm{i}}{2}\sqrt{t}Y_2\cos\phi_2\right) \tag{15}$$
$$\tag{16}$$

$$\frac{\partial}{\partial\theta_y}\Big(\Phi^\dagger(\phi_1,\phi_2)B_{12}^\dagger(t)D_2(\theta_x,\theta_y)B_{12}(t)\Phi(\phi_1,\phi_2)\Big)\Big|_{\theta=0} \tag{17}$$
$$=\left(-\frac{\mathrm{i}}{2}\sqrt{1-t}X_1\cos\phi_1+\frac{\mathrm{i}}{2}\sqrt{1-t}Y_1\sin\phi_1\right)+\left(\frac{\mathrm{i}}{2}\sqrt{t}X_2\cos\phi_2-\frac{\mathrm{i}}{2}\sqrt{t}Y_2\sin\phi_2\right) \tag{18}$$

## II. HOLEVO CRAMÉR-RAO BOUND FOR A SINGLE-MODE PROBE

Starting with the squeezed state $|S(r_1)\rangle = S(r_1)|0\rangle$, we apply a phase rotation $\phi_1$ and pass the state through the displacement channel to get the probe

$$D(\theta_x,\theta_y)\Phi(\phi_1)|S(r_1)\rangle\ . \tag{19}$$

To compute the Holevo-CR bound, we first rotate the probe state by $-\phi_1$. This is done to simplify the computations, it is a unitary transformation which does not change the bound as it can be absorbed as part of the optimal measurement. The rotated probe state is then

$$|\psi_\theta\rangle = \Phi^\dagger(\phi_1)D(\theta_x,\theta_y)\Phi(\phi_1)|S(r_1)\rangle \tag{20}$$
$$= D(\theta_x\cos\phi_1+\theta_y\sin\phi_1,\theta_y\cos\phi_1-\theta_x\sin\phi_1)|S(r_1)\rangle\ . \tag{21}$$

### A. Inner products between the probe and its derivatives

The probe state at $\theta=0$ is

$$|\psi_0\rangle = |S(r_1)\rangle\ . \tag{22}$$

Using Eqns. (2) and (3), differentiation $|\psi_\theta\rangle$ with respect to $\theta_x$ and $\theta_y$, we get

$$|\psi_x\rangle = \frac{\partial}{\partial\theta_x}|\psi_\theta\rangle\Big|_{\theta=0} \tag{23}$$
$$= \left(-\frac{\mathrm{i}}{2}X\sin\phi_1 - \frac{i}{2}Y\cos\phi_1\right)|S(r_1)\rangle\ , \tag{24}$$

and

$$|\psi_y\rangle = \frac{\partial}{\partial\theta_y}|\psi_\theta\rangle\Big|_{\theta=0} \tag{25}$$
$$= \left(\frac{\mathrm{i}}{2}X\cos\phi_1 - \frac{i}{2}Y\sin\phi_1\right)|S(r_1)\rangle\ , \tag{26}$$

Using Eqns. (7) and (8), the inner products between $|\psi_x\rangle$ and $|\psi_y\rangle$ are

$$\langle\psi_x|\psi_x\rangle = \frac{v_{1y}}{4}\ , \tag{27}$$
$$\langle\psi_y|\psi_y\rangle = \frac{v_{1x}}{4}\ , \tag{28}$$

and

$$\langle\psi_x|\psi_y\rangle = \frac{\mathrm{i}+\sinh(2r_1)\sin(2\phi_1)}{4} \tag{29}$$
$$= \frac{\sqrt{v_{1x}v_{1y}}}{4}e^{\mathrm{i}\varphi} \tag{30}$$

where

$$v_{1y} = e^{-2r_1}\sin^2\phi_1 + e^{2r_1}\cos^2\phi_1\ , \tag{31}$$
$$v_{1x} = e^{-2r_1}\cos^2\phi_1 + e^{2r_1}\sin^2\phi_1 \tag{32}$$
$$\tag{33}$$

are the projected variances of the rotated probe on the $X$ and $Y$ quadratures and the angle $\varphi$ satisfies

$$\cos\varphi = \frac{\sinh(2r_1)\sin(2\phi_1)}{\sqrt{v_{1x}v_{1y}}} \tag{34}$$
$$= \mathrm{sign}(r_1\tan\phi_1)\frac{\sqrt{v_{1x}v_{1y}-1}}{\sqrt{v_{1x}v_{1y}}}\ , \tag{35}$$
$$\sin\varphi = \frac{1}{\sqrt{v_{1x}v_{1y}}}\ . \tag{36}$$

Together, the inner products between $|\psi_0\rangle$, $|\psi_x\rangle$ and $|\psi_y\rangle$ are

$$\langle\psi_j|\psi_k\rangle = \begin{pmatrix}1 & 0 & 0\\ 0 & \frac{1}{4}v_{1y} & \frac{1}{4}\sqrt{v_{1x}v_{1y}}e^{\mathrm{i}\varphi}\\ 0 & \frac{1}{4}\sqrt{v_{1x}v_{1y}}e^{-\mathrm{i}\varphi} & \frac{1}{4}v_{1x}\end{pmatrix}\ , \tag{37}$$

for $\{j,k\}\in\{0,x,y\}$. Note that the determinant of this matrix is zero because $|\psi_x\rangle$ and $|\psi_y\rangle$ are in fact linearly dependent. To proceed, we introduce a basis and write

$$|\psi_0\rangle = \begin{pmatrix}1\\0\end{pmatrix} \tag{38}$$
$$|\psi_x\rangle = \frac{\sqrt{v_{1y}}e^{-\mathrm{i}\varphi/2}}{2}\begin{pmatrix}0\\1\end{pmatrix} \tag{39}$$
$$|\psi_y\rangle = \frac{\sqrt{v_{1x}}e^{\mathrm{i}\varphi/2}}{2}\begin{pmatrix}0\\1\end{pmatrix} \tag{40}$$

### B. Computation of the $Z$ matrix

In this basis, after applying the conditions

$$\mathrm{tr}\left\{\rho_\theta \mathcal{X}_j\right\}\big|_{\theta=0} = 0\ , \tag{41}$$

$$\mathrm{tr}\left\{\frac{\partial \rho_\theta}{\partial \theta_j}\mathcal{X}_k\right\}\bigg|_{\theta=0} = \delta_{jk}\ , \tag{42}$$

for $j, k \in \{x, y\}$, the relevant entries for the two matrices $\mathcal{X}_x$ and $\mathcal{X}_y$ are fully determined with

$$\mathcal{X}_x = \begin{pmatrix} 0 & x \\ \bar{x} & \cdot \end{pmatrix} \tag{43}$$

$$\mathcal{X}_y = \begin{pmatrix} 0 & y \\ \bar{y} & \cdot \end{pmatrix} \tag{44}$$

where

$$x = \frac{1}{2\sqrt{v_{1y}}}\left(\frac{1}{\cos(\varphi/2)} + \mathrm{i}\frac{1}{\sin(\varphi/2)}\right) \tag{45}$$

$$y = \frac{1}{2\sqrt{v_{1x}}}\left(\frac{1}{\cos(\varphi/2)} - \mathrm{i}\frac{1}{\sin(\varphi/2)}\right)\ . \tag{46}$$

Substituting this into $Z_\theta[\mathcal{X}]_{jk} := \mathrm{tr}\left\{\rho_\theta \mathcal{X}_j \mathcal{X}_k\right\}$, we get

$$Z = \begin{pmatrix} |x|^2 & x\,\bar{y} \\ \bar{x}y & |y|^2 \end{pmatrix} \tag{47}$$

$$= \begin{pmatrix} v_{1x} & -\sinh(2r_1)\sin(2\phi) + \mathrm{i} \\ -\sinh(2r_1)\sin(2\phi) - \mathrm{i} & v_{1y} \end{pmatrix} \tag{48}$$

which does not depend on $\varphi$.

### C. Holevo-CR bound for a fixed weight matrix

With a diagonal weighting matrix

$$W = \begin{pmatrix} w_x & 0 \\ 0 & w_y \end{pmatrix}\ , \tag{49}$$

the function

$$h = \mathrm{Tr}\left\{W\,\mathrm{Re}Z\right\} + \left\|\sqrt{W}\,\mathrm{Im}Z\,\sqrt{W}\right\|_1 \tag{50}$$

$$= w_x v_{1x} + w_y v_{1y} + 2\sqrt{w_x w_y}\ . \tag{51}$$

Hence the Holevo-CR bound is

$$w_x v_x + w_y v_y \geq w_x v_{1x} + w_y v_{1y} + 2\sqrt{w_x w_y}\ . \tag{52}$$

Each value of $w_x$ and $w_y$ in Eqn. (52) restricts the values $v_x$ and $v_y$ can take. For some values of $w_x$ and $w_y$, we get

$$(w_x = w_y = 1) : v_x + v_y \geq v_{1x} + v_{1y} + 2 = 2(1 + \cosh 2r_1) \tag{53}$$

$$(w_x = 1, w_y = 0) : v_x \geq v_{1x} \tag{54}$$

$$(w_x = 0, w_y = 1) : v_y \geq v_{1y} \tag{55}$$

### D. Collecting all the bounds with different weighting matrix

To find all the possible values for $v_x$ and $v_y$, we look for the solutions to Eqn. (52) valid for all $w_x$ and $w_y$. Rearranging Eqn. (52), we have

$$w(v_y - v_{1y}) - 2\sqrt{w} + (v_x - v_{1x}) \geq 0 \tag{56}$$

where $w = w_y/w_x$. This is a quadratic equation in $\sqrt{w}$ and the statement is true for all $w$ if and only if

$$4 - 4(v_y - v_{1y})(v_x - v_{1x}) \leq 0 \tag{57}$$
$$\Rightarrow (v_y - v_{1y})(v_x - v_{1x}) \geq 1 \tag{58}$$

where we already know from Eqns. (54) and (55) that $v_x \geq v_{1x}$ and $v_y \geq v_{1y}$.

### E. Optimising the rotation angle $\phi$

For every rotation angle $\phi$, and $v_x > v_{1x}$, Eqn. (58) gives the smallest value of $v_y$ as

$$v_y = v_{1y} + \frac{1}{v_x - v_{1x}} \, . \tag{59}$$

Finally, we want to find the rotation angle that minimises $v_y$ for a fixed $v_x$. Without any loss of generality, we can consider $r_1 > 0$ so that $v_x > e^{-2r_1}$. Performing the minimisation, we find

$$v_y^* = \min_{\phi} \left\{ v_{1y} + \frac{1}{v_x - v_{1x}} \right\} \text{ subject to } v_{1x} \leq v_x \tag{60}$$

$$= \begin{cases} e^{2r_1} + \dfrac{1}{v_x - e^{-2r_1}} & \text{at } \phi = 0 & \text{if } e^{-2r_1} \leq v_x < 1 + e^{-2r_1} \\ 2 + 2\cosh 2r_1 - v_x & \text{at } \phi = \arccos\left(\dfrac{e^r\sqrt{1+e^{2r_1} - v_x}}{\sqrt{e^{4r}-1}}\right) & \text{if } 1 + e^{-2r_1} \leq v_x < 1 + e^{2r_1} \\ e^{-2r_1} + \dfrac{1}{v_x - e^{2r_1}} & \text{at } \phi = \pi/2 & \text{if } v_x \geq 1 + e^{2r_1} \end{cases} \tag{61}$$

which is plotted in Fig. 1.

## III. HOLEVO CRAMÉR-RAO BOUND FOR A TWO-MODE PROBE

An arbitrary two-mode passive linear optical network can be realised by two phase-shifts at the input port, a beam-splitter and a phase-shift at one of the exit port. The phase shift on the exit port can be placed on the mode that is not the probe. Hence this does not have any effect on the estimation precision because it can be undone in the measurement stage. Therefore, starting with the two squeezed states $|S(r_1, r_2)\rangle = S(r_1) \otimes S(r_2) |0, 0\rangle$, it is sufficient to consider just two rotations $\phi_1$ and $\phi_2$ on each, and mix them through a beam-splitter with splitting ratio $t$ as the most general passive linear operation. The probe state is then

$$D_2(\theta_x, \theta_y) B_{12}(t) \Phi(\phi_1, \phi_2) |S(r_1, r_2)\rangle \, . \tag{62}$$

To compute the Holevo-CR bound, we first undo the mixing and rotation operation on the probe state by performing $B_{12}(t)$ and $\Phi(\phi_1, \phi_2)$ in reverse. Once again, this is done to simplify the computations, it is a unitary transformation which does not change the bound as it can be absorbed as part of the optimal measurement. The two-mode probe state is then

$$|\psi_\theta\rangle = \Phi^\dagger(\phi_1, \phi_2) B_{12}^\dagger(t) D_2(\theta_x, \theta_y) B_{12}(t) \Phi(\phi_1, \phi_2) |S(r_1, r_2)\rangle \, . \tag{63}$$

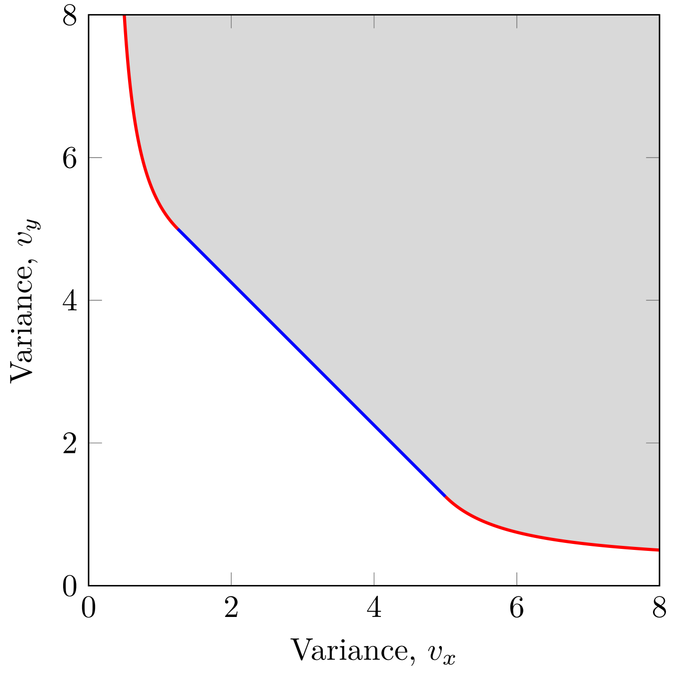


FIG. 1. The three line segments plots Eqns. (60) which give the minimum estimator variance $v_y$ that can be attained for a given $v_x$ using a squeezed probe with a squeezed variance of $r_1 = 0.69$. The grey shaded region shows the accessible areas.

### A. Inner products between the probe and its derivatives

The probe state at $\theta = 0$ is

$$|\psi_0\rangle = |S(r_1, r_2)\rangle \ . \tag{64}$$

Using Eqns. (15) and (18), we can differentiate $|\psi_\theta\rangle$ with respect to $\theta_x$ and $\theta_y$ to get

$$|\psi_x\rangle = \frac{\partial}{\partial\theta_x} |\psi_\theta\rangle\Big|_{\theta=0} \tag{65}$$

$$= \left(\frac{\mathrm{i}}{2}\sqrt{1-t}X_1 \sin\phi_1 + \frac{\mathrm{i}}{2}\sqrt{1-t}Y_1 \cos\phi_1\right)|S(r_1, r_2)\rangle + \left(-\frac{\mathrm{i}}{2}\sqrt{t}X_2 \sin\phi_2 - \frac{\mathrm{i}}{2}\sqrt{t}Y_2 \cos\phi_2\right)|S(r_1, r_2)\rangle \ , \tag{66}$$

and

$$|\psi_y\rangle = \frac{\partial}{\partial\theta_y} |\psi_\theta\rangle\Big|_{\theta=0} \tag{67}$$

$$= \left(-\frac{\mathrm{i}}{2}\sqrt{1-t}X_1 \cos\phi_1 + \frac{\mathrm{i}}{2}\sqrt{1-t}Y_1 \sin\phi_1\right)|S(r_1, r_2)\rangle + \left(\frac{\mathrm{i}}{2}\sqrt{t}X_2 \cos\phi_2 - \frac{\mathrm{i}}{2}\sqrt{t}Y_2 \sin\phi_2\right)|S(r_1, r_2)\rangle \ . \tag{68}$$

Using Eqns. (7) and (8), the inner products between $|\psi_x\rangle$ and $|\psi_y\rangle$ are

$$\langle\psi_x|\psi_x\rangle = \frac{1-t}{4}v_{1y} + \frac{t}{4}v_{2y} \ , \tag{69}$$

$$\langle\psi_y|\psi_y\rangle = \frac{1-t}{4}v_{1x} + \frac{t}{4}v_{2x} \ , \tag{70}$$

and

$$\langle\psi_x|\psi_y\rangle = \frac{i}{4} + \frac{1-t}{4}\sinh(2r_1)\sin(2\phi_1) + \frac{t}{4}\sinh(2r_2)\sin(2\phi_2) \tag{71}$$

$$= \frac{1-t}{4}\sqrt{v_{1x}v_{1y}}e^{\mathrm{i}\varphi_1} + \frac{t}{4}\sqrt{v_{2x}v_{2y}}e^{\mathrm{i}\varphi_2} \tag{72}$$

where

$$v_{1y} = e^{-2r_1}\sin^2\phi_1 + e^{2r_1}\cos^2\phi_1 \ , \tag{73}$$

$$v_{1x} = e^{-2r_1}\cos^2\phi_1 + e^{2r_1}\sin^2\phi_1 \ , \tag{74}$$

$$v_{2y} = e^{-2r_2}\sin^2\phi_2 + e^{2r_2}\cos^2\phi_2 \ , \tag{75}$$

$$v_{2x} = e^{-2r_2}\cos^2\phi_2 + e^{2r_2}\sin^2\phi_2 \tag{76}$$

are the projected variances of the rotated probe on the $X$ and $Y$ quadratures and the angles $\varphi_1$ and $\varphi_2$ satisfy

$$\cos\varphi_1 = \frac{\sinh(2r_1)\sin(2\phi_1)}{\sqrt{v_{1x}v_{1y}}} \tag{77}$$

$$= \mathrm{sign}(r_1\tan\phi_1)\frac{\sqrt{v_{1x}v_{1y}-1}}{\sqrt{v_{1x}v_{1y}}} \ , \tag{78}$$

$$\sin\varphi_1 = \frac{1}{\sqrt{v_{1x}v_{1y}}} \ , \tag{79}$$

$$\cos\varphi_2 = \frac{\sinh(2r_2)\sin(2\phi_2)}{\sqrt{v_{2x}v_{2y}}} \tag{80}$$

$$= \mathrm{sign}(r_2\tan\phi_2)\frac{\sqrt{v_{2x}v_{2y}-1}}{\sqrt{v_{2x}v_{2y}}} \ , \tag{81}$$

$$\sin\varphi_2 = \frac{1}{\sqrt{v_{2x}v_{2y}}} \ . \tag{82}$$

Together, the inner products between $|\psi_0\rangle$, $|\psi_x\rangle$ and $|\psi_y\rangle$ are

$$\langle\psi_j|\psi_k\rangle = \begin{pmatrix} 1 & 0 & 0 \\ 0 & \frac{1-t}{4}v_{1y} + \frac{t}{4}v_{2y} & \frac{1-t}{4}\sqrt{v_{1x}v_{1y}}e^{\mathrm{i}\varphi_1} + \frac{t}{4}\sqrt{v_{2x}v_{2y}}e^{\mathrm{i}\varphi_2} \\ 0 & \frac{1-t}{4}\sqrt{v_{1x}v_{1y}}e^{-\mathrm{i}\varphi_1} + \frac{t}{4}\sqrt{v_{2x}v_{2y}}e^{-\mathrm{i}\varphi_2} & \frac{1-t}{4}v_{1x} + \frac{t}{4}v_{2x} \end{pmatrix} \ , \tag{83}$$

for $\{j,k\} \in \{0,x,y\}$. To proceed, we introduce a basis and write

$$|\psi_0\rangle = \begin{pmatrix} 1 \\ 0 \\ 0 \end{pmatrix} \tag{84}$$

$$|\psi_x\rangle = \frac{1}{2}\begin{pmatrix} 0 \\ \sqrt{1-t}\sqrt{v_{1y}}e^{-\mathrm{i}\varphi_1/2} \\ \sqrt{t}\sqrt{v_{2y}}e^{-\mathrm{i}\varphi_2/2} \end{pmatrix} \tag{85}$$

$$|\psi_y\rangle = \frac{1}{2}\begin{pmatrix} 0 \\ \sqrt{1-t}\sqrt{v_{1x}}e^{\mathrm{i}\varphi_1/2} \\ \sqrt{t}\sqrt{v_{2x}}e^{\mathrm{i}\varphi_2/2} \end{pmatrix} \ . \tag{86}$$

### B. Computation of the $Z$ matrix

In this basis, after applying the conditions

$$\mathrm{tr}\left\{\rho_\theta \mathcal{X}_j\right\}\big|_{\theta=0} = 0 \ , \tag{87}$$

$$\mathrm{tr}\left\{\frac{\partial\rho_\theta}{\partial\theta_j}\mathcal{X}_k\right\}\bigg|_{\theta=0} = \delta_{jk} \ , \tag{88}$$

for $j,k \in \{x,y\}$, we can write the relevant entries for the two matrices $\mathcal{X}_x$ and $\mathcal{X}_y$ as

$$\mathcal{X}_x = \begin{pmatrix} 0 & x_1 e^{\mathrm{i}\varphi_1/2} & x_2 e^{\mathrm{i}\varphi_2/2} \\ \bar{x}_1 e^{-\mathrm{i}\varphi_1/2} & \cdot & \cdot \\ \bar{x}_2 e^{-\mathrm{i}\varphi_2/2} & \cdot & \cdot \end{pmatrix} , \tag{89}$$

$$\mathcal{X}_y = \begin{pmatrix} 0 & y_1 e^{\mathrm{i}\varphi_1/2} & y_2 e^{\mathrm{i}\varphi_2/2} \\ \bar{y}_1 e^{-\mathrm{i}\varphi_1/2} & \cdot & \cdot \\ \bar{y}_2 e^{-\mathrm{i}\varphi_2/2} & \cdot & \cdot \end{pmatrix} , \tag{90}$$

where the complex entries $x_1$, $x_2$, $y_1$ and $y_2$ must satisfy the constraints

$$\sqrt{1-t}\sqrt{v_{1y}}\,\mathrm{Re}\,\{x_1\} + \sqrt{t}\sqrt{v_{2y}}\,\mathrm{Re}\,\{x_2\} = 1 , \tag{91}$$

$$\sqrt{1-t}\sqrt{v_{1x}}\,\mathrm{Re}\,\{x_1 e^{\mathrm{i}\varphi_1}\} + \sqrt{t}\sqrt{v_{2x}}\,\mathrm{Re}\,\{x_2 e^{\mathrm{i}\varphi_2}\} = 0 , \tag{92}$$

$$\sqrt{1-t}\sqrt{v_{1y}}\,\mathrm{Re}\,\{y_1\} + \sqrt{t}\sqrt{v_{2y}}\,\mathrm{Re}\,\{y_2\} = 0 , \tag{93}$$

$$\sqrt{1-t}\sqrt{v_{1x}}\,\mathrm{Re}\,\{y_1 e^{\mathrm{i}\varphi_1}\} + \sqrt{t}\sqrt{v_{2x}}\,\mathrm{Re}\,\{y_2 e^{\mathrm{i}\varphi_2}\} = 1 . \tag{94}$$

Substituting this into $Z_\theta[\mathcal{X}]_{jk} {:=} \mathrm{tr}\,\{\rho_\theta \mathcal{X}_j \mathcal{X}_k\}$, we get

$$Z = \begin{pmatrix} |x_1|^2 + |x_2|^2 & x_1\bar{y}_1 + x_2\bar{y}_2 \\ \bar{x}_1 y_1 + \bar{x}_2 y_2 & |y_1|^2 + |y_2|^2 \end{pmatrix} . \tag{95}$$

### C. Computation for the Holevo-CR bound

With a diagonal weighting matrix

$$W = \begin{pmatrix} w_x & 0 \\ 0 & w_y \end{pmatrix} , \tag{96}$$

the function $h$ can be written as

$$h = \mathrm{Tr}\,\{W\,\mathrm{Re}Z\} + \left\|\sqrt{W}\,\mathrm{Im}Z\sqrt{W}\right\|_1 \tag{97}$$

$$= w_x \underbrace{\left(|x_1|^2 + |x_2|^2\right)}_{f_x} + w_y \underbrace{\left(|y_1|^2 + |y_2|^2\right)}_{f_y} + 2\sqrt{w_x w_y}\,\mathrm{Abs}\{\underbrace{\mathrm{Im}\,\{x_1\bar{y}_1 + x_2\bar{y}_2\}}_{g}\} . \tag{98}$$

The Holevo-CR bound is obtained by the following minimisation

$$w_x v_x + w_y v_y \geq f_{\mathrm{HCR}} := \min_{x_1,x_2,y_1,y_2} h \tag{99}$$

subject to the four constraints (91)–(94). When the probe parameters $r_1$, $r_2$, $\phi_1$, $\phi_2$ and $t$ as well as the weights $w_x$ and $w_y$ are specified, this is an instance of a semidefinite programme which can be solved efficiently using numerical methods. Furthermore, every semidefinite programme has a dual problem which can be used to verify the minimisation solution. The minimum point occurs when $g = 0$ at which we obtain a solution for the extremal point as $v_x = f_x$ and $v_y = f_y$. The locus of the extremal points $(v_x, v_y)$ as we vary the ratio $w_x/w_y$ from 0 to infinity gives the boundary of the accessible region for a specified probe. To find the optimal use of a given resource characterised by $r_1$ and $r_2$, we need to further minimise $f_{\mathrm{HCR}}$ over the parameters $\phi_1$, $\phi_2$ and $t$. This is what we have done to plot Fig. 2 of the main text.

While solving the semidefinite programme can give us numerical solutions, we can also solve the minimisation problem by solving for the Karush-Kuhn-Tucker conditions for optimality.

### D. Proof of main result

In what follows, we provide a proof our main result. We break up the proof into four steps. First, we prove that $h$ is minimised when $g = 0$. Second, we provide numerical evidence that $f_{\mathrm{HCR}}$ is minimised when $\phi_1$ and $\phi_2$ are either 0 or $\pi/2$. Third, we compute the Holevo-CR bound for a fixed $t$. Lastly, we vary $t$ to find all the accessible values for $v_x$ and $v_y$.

### 1. Observation 1: $h$ is minimised when $g = 0$

We claim that $h$ in Eq. (97) is minimised when $g = 0$. To proof this claim, we first introduce the rescaled variables

$$\mathsf{x}_1 = \sqrt{w_x}x_1\,,\ \mathsf{x}_2 = \sqrt{w_x}x_2\,,\ \mathsf{y}_1 = \sqrt{w_y}y_1\,,\ \mathsf{y}_2 = \sqrt{w_y}y_2\,. \tag{100}$$

In the rescaled variables, function to be minimised Eq. (97) can be written as

$$h = |\mathsf{x}_1|^2 + |\mathsf{x}_2|^2 + |\mathsf{y}_1|^2 + |\mathsf{y}_2|^2 + 2\,\mathrm{Abs}\Big\{\mathrm{Im}\left\{\mathsf{x}_1\bar{\mathsf{y}}_1 + \mathsf{x}_2\bar{\mathsf{y}}_2\right\}\Big\} \tag{101}$$

$$= \max\left\{\,|\vec{\mathsf{x}}+\vec{\mathsf{y}}|^2\,,\,|\vec{\mathsf{x}}-\vec{\mathsf{y}}|^2\,\right\}, \tag{102}$$

where

$$\vec{\mathsf{x}} = \begin{pmatrix}\mathrm{Re}\,\mathsf{x}_1 & \mathrm{Im}\,\mathsf{x}_1 & \mathrm{Re}\,\mathsf{y}_2 & \mathrm{Im}\,\mathsf{y}_2\end{pmatrix}^{\intercal}\,, \tag{103}$$

$$\vec{\mathsf{y}} = \begin{pmatrix}-\mathrm{Im}\,\mathsf{y}_1 & \mathrm{Re}\,\mathsf{y}_1 & \mathrm{Im}\,\mathsf{x}_2 & -\mathrm{Re}\,\mathsf{x}_2\end{pmatrix}^{\intercal}\,. \tag{104}$$

Our claim is then: $h$ is minimised when $\vec{\mathsf{x}}\cdot\vec{\mathsf{y}} = 0$. We can write the constraints (91)–(94) as

$$\begin{pmatrix}c_1 & 0\\ c_3 & c_4\end{pmatrix}\begin{pmatrix}\mathrm{Re}\,\mathsf{x}_1\\ \mathrm{Im}\,\mathsf{x}_1\end{pmatrix} + \begin{pmatrix}0 & -c_2\\ c_6 & -c_5\end{pmatrix}\begin{pmatrix}\mathrm{Im}\,\mathsf{x}_2\\ -\mathrm{Re}\,\mathsf{x}_2\end{pmatrix} = \begin{pmatrix}\sqrt{w_x}\\ 0\end{pmatrix}, \tag{105}$$

$$\begin{pmatrix}0 & c_1\\ -c_4 & c_3\end{pmatrix}\begin{pmatrix}-\mathrm{Im}\,\mathsf{y}_1\\ \mathrm{Re}\,\mathsf{y}_1\end{pmatrix} + \begin{pmatrix}c_2 & 0\\ c_5 & c_6\end{pmatrix}\begin{pmatrix}\mathrm{Re}\,\mathsf{y}_2\\ \mathrm{Im}\,\mathsf{y}_2\end{pmatrix} = \begin{pmatrix}0\\ \sqrt{w_y}\end{pmatrix} \tag{106}$$

where

$$c_1 = \sqrt{1-t}\sqrt{v_{1y}}\,,\ c_3 = \sqrt{1-t}\sqrt{v_{1x}}\cos\varphi_1\,,\quad c_5 = \sqrt{t}\sqrt{v_{2x}}\cos\varphi_2\,, \tag{107}$$

$$c_2 = \sqrt{t}\sqrt{v_{2y}}\,,\quad c_4 = -\sqrt{1-t}\sqrt{v_{1x}}\sin\varphi_1\,,\ c_6 = -\sqrt{t}\sqrt{v_{2x}}\sin\varphi_2\,. \tag{108}$$

We can invert these equations to find $\vec{\mathsf{y}}$ in terms of $\vec{\mathsf{x}}$

$$\begin{pmatrix}-\mathrm{Im}\,\mathsf{y}_1\\ \mathrm{Re}\,\mathsf{y}_1\end{pmatrix} = \begin{pmatrix}0 & c_1\\ -c_4 & c_3\end{pmatrix}^{-1}\begin{pmatrix}0\\ \sqrt{w_y}\end{pmatrix} - \begin{pmatrix}0 & c_1\\ -c_4 & c_3\end{pmatrix}^{-1}\begin{pmatrix}c_2 & 0\\ c_5 & c_6\end{pmatrix}\begin{pmatrix}\mathrm{Re}\,\mathsf{y}_2\\ \mathrm{Im}\,\mathsf{y}_2\end{pmatrix}, \tag{109}$$

$$\begin{pmatrix}\mathrm{Im}\,\mathsf{x}_2\\ -\mathrm{Re}\,\mathsf{x}_2\end{pmatrix} = \begin{pmatrix}0 & -c_2\\ c_6 & -c_5\end{pmatrix}^{-1}\begin{pmatrix}\sqrt{w_x}\\ 0\end{pmatrix} - \begin{pmatrix}0 & -c_2\\ c_6 & -c_5\end{pmatrix}^{-1}\begin{pmatrix}c_1 & 0\\ c_3 & c_4\end{pmatrix}\begin{pmatrix}\mathrm{Re}\,\mathsf{x}_1\\ \mathrm{Im}\,\mathsf{x}_1\end{pmatrix} \tag{110}$$

whenever the matrices $\begin{pmatrix}0 & c_1\\ -c_4 & c_3\end{pmatrix}$ and $\begin{pmatrix}0 & -c_2\\ c_6 & -c_5\end{pmatrix}$ are invertible. This is always true when $t$ is not exactly 0 or 1 in which case we can write $\vec{\mathsf{y}} = \mathbb{A}\vec{\mathsf{x}} + \vec{b}$ where

$$\mathbb{A} = -\begin{pmatrix}\begin{pmatrix}0 & c_1\\ -c_4 & c_3\end{pmatrix}^{-1} & \mathbb{0}\\ \mathbb{0} & \begin{pmatrix}0 & -c_2\\ c_6 & -c_5\end{pmatrix}^{-1}\end{pmatrix}\begin{pmatrix}\mathbb{0} & \begin{pmatrix}c_2 & 0\\ c_5 & c_6\end{pmatrix}\\ \begin{pmatrix}c_1 & 0\\ c_3 & c_4\end{pmatrix} & \mathbb{0}\end{pmatrix}\ \text{and} \tag{111}$$

$$\vec{b} = \begin{pmatrix}\begin{pmatrix}0 & c_1\\ -c_4 & c_3\end{pmatrix}^{-1} & \mathbb{0}\\ \mathbb{0} & \begin{pmatrix}0 & -c_2\\ c_6 & -c_5\end{pmatrix}^{-1}\end{pmatrix}\begin{pmatrix}0\\ \sqrt{w_y}\\ \sqrt{w_x}\\ 0\end{pmatrix}. \tag{112}$$

Given $\vec{\mathsf{x}}$, the vector $\vec{\mathsf{y}}$ is fixed which means we can perform an unconstrained minimisation over $\vec{\mathsf{x}}$ only

$$f_{\mathrm{HCR}} = \min_{\vec{\mathsf{x}}}\max\left\{\,|\vec{\mathsf{x}}+\vec{\mathsf{y}}|^2\,,\,|\vec{\mathsf{x}}-\vec{\mathsf{y}}|^2\,\right\}. \tag{113}$$

Because $f_{\mathrm{HCR}}$ is continuous in $\vec{\mathsf{x}}$ and bounded below by zero, it has a minimum. To proof our claim we shall show that the alternative statement: "$h$ is minimised when $\vec{\mathsf{x}}\cdot\vec{\mathsf{y}} \neq 0$." leads to a contradiction. Suppose $h$ is minimised by $\vec{\mathsf{x}}_\star$ and its corresponding $\vec{\mathsf{y}}_\star$ such that $\vec{\mathsf{x}}_\star\cdot\vec{\mathsf{y}}_\star > 0$. This implies

$$f_{\mathrm{HCR}} = \min_{\vec{\mathsf{x}}}|\vec{\mathsf{x}}+\vec{\mathsf{y}}|^2\,. \tag{114}$$

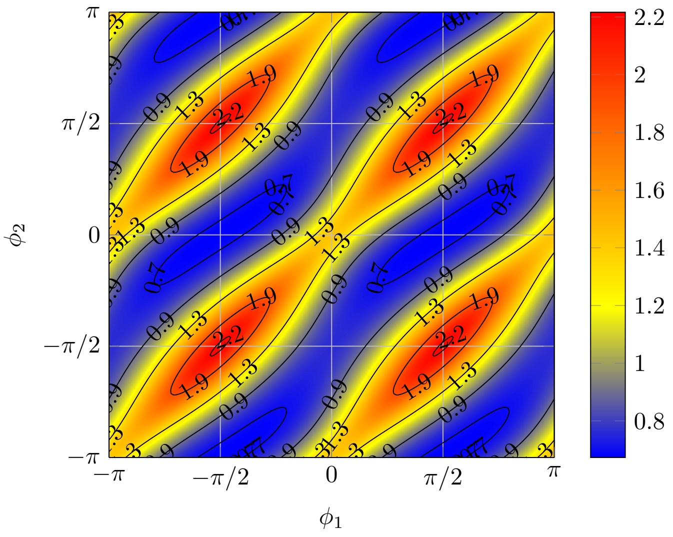

FIG. 2. A typical contour plot of $f_{\mathrm{HCR}}$ for a fixed $r_1 = 0.35$, $r_2 = 0.69$, $t = 0.4$, $w_x = 0.7$ and $w_y = 0.3$ as we scan the angles $\phi_1$ and $\phi_2$. In this case, $f_{\mathrm{HCR}}$ is minimised when $\phi_1 = \pi/2$ and $\phi_2 = 0$.

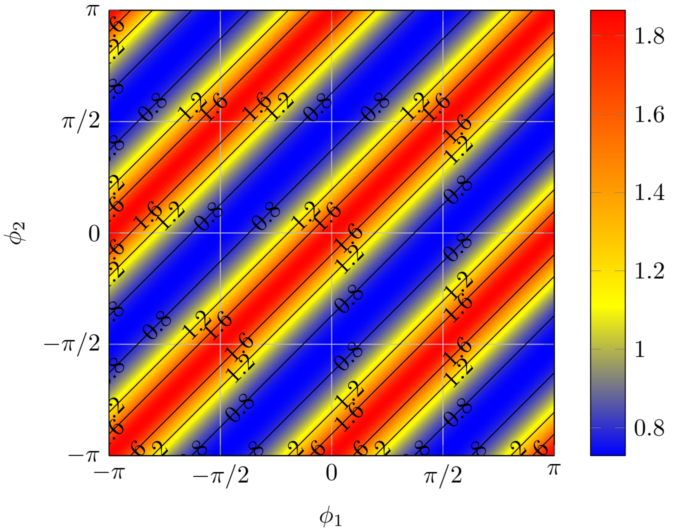

FIG. 3. When $w_x = w_y = 0.5$, a typical contour plot of $f_{\mathrm{HCR}}$ for a fixed $r_1 = 0.35$, $r_2 = 0.69$ and $t = 0.4$ as we scan the angles $\phi_1$ and $\phi_2$. In this case, $f_{\mathrm{HCR}}$ is minimised when $\phi_2 = \phi_1 + \pi/2$.

However, the function $|\vec{\mathsf{x}} + \vec{\mathsf{y}}|^2$ attains a minimum of zero when

$$\vec{\mathsf{x}}_+ = -\left(\mathbb{A} + \mathbb{1}\right)^{-1} \vec{b} \tag{115}$$

such that $\vec{\mathsf{y}}_+ = -\vec{\mathsf{x}}_+$ which implies $\vec{\mathsf{x}}_+ \cdot \vec{\mathsf{y}}_+ = -\left|\vec{\mathsf{x}}_+\right|^2 \leq 0$ leading to a contradiction. Following a similar argument, supposing $\vec{\mathsf{x}}_\star \cdot \vec{\mathsf{y}}_\star < 0$ also leads to a contradiction. Since the minimum cannot occur when $\vec{\mathsf{x}} \cdot \vec{\mathsf{y}} \neq 0$, at the minimum point, we must have $\vec{\mathsf{x}} \cdot \vec{\mathsf{y}} = 0$ which proves our claim. Hence, we can write the Holevo-CR bound as

$$f_{\mathrm{HCR}} = \min_{\vec{\mathsf{x}}} \left|\vec{\mathsf{x}} + \vec{\mathsf{y}}\right|^2 \ , \text{ subject to } \vec{\mathsf{x}} \cdot \vec{\mathsf{y}} = 0 \ . \tag{116}$$

### 2. *Step 2: Numerical evidence that the minimum can be attained when $\phi_1 = 0$ and $\phi_2 = \pi/2$ or $\phi_1 = \pi/2$ and $\phi_2 = 0$*

For any given values of $r_1$, $r_2$, $t$, $w_x$ and $w_y$, we conjecture that the minimum for $h$ can always be attained when $\phi_1 = 0$ and $\phi_2 = \pi/2$ or when $\phi_1 = \pi/2$ and $\phi_2 = 0$. For each value of $\phi_1$ and $\phi_2$ we can solve a semi-definite program

to find the minimum $f_{\rm HCR}(\phi_1, \phi_2)$. We can then scan over the angles $\phi_1$ and $\phi_2$ to look for the minimum $f_{\rm HCR}$. Doing this, we find that the minimum of $f_{\rm HCR}$ always occur when $\phi_1$ and $\phi_2$ are equal to either 0 or $\pi/2$. A simulation for a typical setting with $r_1 = 0.35$, $r_2 = 0.69$, $t = 0.4$, $w_x = 0.7$ and $w_y = 0.3$ is shown in Fig. 2.

In the special case when $w_x = w_y$, we find that any value every value of $\phi_1$ and $\phi_2$ satisfying $\phi_2 = \phi_1 + \pi/2$ gives the same optimal $f_{\rm HCR}$. A typical simulation result is shown in Fig. 3.

### 3. *Step 3: Minimizing $h$ for a fixed $w_x$, $w_y$ and $t$, when $\phi_1$ and $\phi_2$ are equal to 0 or $\pi/2$*

When $\phi_1$ and $\phi_2$ are equal 0 or $\pi/2$ the products $v_{1x}v_{1y} = v_{2x}v_{2y} = 1$ and $\varphi_1 = \varphi_2 = \pi/2$. This simplifies the inner products between the states of interest to

$$\langle\psi_j|\psi_k\rangle = \begin{pmatrix} 1 & 0 & 0 \\ 0 & \frac{1-t}{4}v_{1y} + \frac{t}{4}v_{2y} & \frac{i}{4} \\ 0 & -\frac{i}{4} & \frac{1-t}{4}v_{1x} + \frac{t}{4}v_{2x} \end{pmatrix} . \tag{117}$$

The coefficients $c_3 = c_5 = 0$, $c_4 = -\sqrt{1-t}\sqrt{v_{1x}}$ and $c_6 = -\sqrt{t}\sqrt{v_{2x}}$ in Eqns. (105)–(106). The matrix $\mathbb{A}$ and vector $\vec{b}$ relating $\vec{\mathsf{y}}$ and $\vec{\mathsf{x}}$ are now

$$\mathbb{A} = -\begin{pmatrix} 0 & 0 & 0 & c_6/c_4 \\ 0 & 0 & -c_2/c_1 & 0 \\ 0 & -c_4/c_6 & 0 & 0 \\ c_1/c_2 & 0 & 0 & 0 \end{pmatrix} \text{ and } \vec{b} = \begin{pmatrix} -\sqrt{w_y}/c_4 \\ 0 \\ 0 \\ -\sqrt{w_x}/c_2 \end{pmatrix} . \tag{118}$$

The relation between the original variables becomes

$$\mathrm{Re}\, x_2 = \frac{1}{c_2}\left(1 - c_1 \mathrm{Re}\, x_1\right) \tag{119}$$
$$\mathrm{Im}\, x_2 = -\frac{c_4}{c_6}\mathrm{Im}\, x_1 \tag{120}$$
$$\mathrm{Re}\, y_1 = -\frac{c_2}{c_1}\mathrm{Re}\, y_2 \tag{121}$$
$$\mathrm{Im}\, y_1 = \frac{1}{c_4}\left(1 - c_6 \mathrm{Re}\, x_1\right) . \tag{122}$$

To compute the Holevo-CR bound (116), we now have to minimise over $x_1$ and $y_2$

$$h = w_x f_x + w_y f_y \tag{123}$$

where

$$f_x = (\mathrm{Re}\, x_1)^2 + (\mathrm{Im}\, x_1)^2 + \left(\frac{1 - c_1\mathrm{Re}\, x_1}{c_2}\right)^2 + \left(\frac{c_4 \mathrm{Im}\, x_1}{c_6}\right)^2 , \tag{124}$$
$$f_y = (\mathrm{Re}\, y_2)^2 + (\mathrm{Im}\, y_2)^2 + \left(\frac{1 - c_6\mathrm{Im}\, y_2}{c_4}\right)^2 + \left(\frac{c_2 \mathrm{Re}\, y_2}{c_1}\right)^2 \tag{125}$$

subject to the condition

$$g = -\mathrm{Im}\, y_1 \mathrm{Re}\, x_1 + \mathrm{Re}\, y_1 \mathrm{Im}\, x_1 + \mathrm{Im}\, x_2 \mathrm{Re}\, y_2 - \mathrm{Re}\, x_2 \mathrm{Im}\, y_2 \tag{126}$$
$$= \frac{\mathrm{Im}\, x_1 \mathrm{Re}\, y_2}{c_1 c_6} - \frac{\mathrm{Re}\, x_1 \mathrm{Im}\, y_2}{c_2 c_4} - \frac{\mathrm{Re}\, x_1}{c_4} - \frac{\mathrm{Im}\, y_2}{c_2} \tag{127}$$
$$= 0 . \tag{128}$$

To find the minimum value of $h$, we introduce the Lagrangian function

$$\mathcal{L} = h + \lambda g \tag{129}$$

where $\lambda$ is the Lagrange multiplier. To find the stationary points for $\mathcal{L}$ we differentiate with respect to $x_1$ and $y_2$ and set them to zero:

$$\frac{\partial \mathcal{L}}{\partial \mathrm{Im}\, x_1} = w_x \left[ 2\mathrm{Im}\, x_1 + \frac{2c_4^2}{c_6^2} \mathrm{Im}\, x_1 \right] + \lambda \left( \frac{\mathrm{Re}\, y_2}{c_1 c_6} \right) = 0 \tag{130}$$

$$\frac{\partial \mathcal{L}}{\partial \mathrm{Re}\, y_2} = w_y \left[ 2\mathrm{Re}\, y_2 + \frac{2c_2^2}{c_1^2} \mathrm{Re}\, y_2 \right] + \lambda \left( \frac{\mathrm{Im}\, x_1}{c_1 c_6} \right) = 0 \tag{131}$$

$$\frac{\partial \mathcal{L}}{\partial \mathrm{Re}\, x_1} = w_x \left[ 2\mathrm{Re}\, x_1 - \frac{2c_1}{c_2} \left( \frac{1 - c_1 \mathrm{Re}\, x_1}{c_2} \right) \right] - \lambda \left( \frac{\mathrm{Im}\, y_2}{c_2 c_4} + \frac{1}{c_4} \right) = 0 \tag{132}$$

$$\frac{\partial \mathcal{L}}{\partial \mathrm{Im}\, y_2} = w_y \left[ 2\mathrm{Im}\, y_2 - \frac{2c_6}{c_4} \left( \frac{1 - c_6 \mathrm{Im}\, y_2}{c_4} \right) \right] - \lambda \left( \frac{\mathrm{Re}\, x_1}{c_2 c_4} + \frac{1}{c_2} \right) = 0 \tag{133}$$

$$\frac{\partial \mathcal{L}}{\partial \lambda} = \frac{\mathrm{Im}\, x_1 \mathrm{Re}\, y_2}{c_1 c_6} - \frac{\mathrm{Re}\, x_1 \mathrm{Im}\, y_2}{c_2 c_4} - \frac{\mathrm{Re}\, x_1}{c_4} - \frac{\mathrm{Im}\, y_2}{c_2} = 0\,. \tag{134}$$

From Eqns. (130)–(131), we have

$$\mathrm{Im}\, x_1 = -\frac{\lambda}{2 w_x c_1 c_6 (1 + c_4^2/c_6^2)} \mathrm{Re}\, y_2 \tag{135}$$

$$\mathrm{Im}\, x_1 = -\frac{2 w_y c_1 c_6 (1 + c_2^2/c_1^2)}{\lambda} \mathrm{Re}\, y_2\,, \tag{136}$$

which implies either of the two cases.

$$\text{Case A: } \mathrm{Re}\, y_2 = \mathrm{Im}\, x_1 = 0\,. \tag{137}$$

$$\text{Case B: } \lambda^2 = 4 w_x w_y c_1^2 c_6^2 \left(1 + \frac{c_2^2}{c_1^2}\right)\left(1 + \frac{c_4^2}{c_6^2}\right) \tag{138}$$

$$= 4 w_x w_y \left(c_1^2 + c_2^2\right)\left(c_4^2 + c_6^2\right) \tag{139}$$

$$\Rightarrow \lambda = \pm \underbrace{2\sqrt{w_x w_y \left(c_1^2 + c_2^2\right)\left(c_4^2 + c_6^2\right)}}_{\lambda_0}\,. \tag{140}$$

From Eqns. (132)–(133), we require

$$\mathrm{Im}\, y_2 = \frac{2 w_x c_4 (c_1^2 + c_2^2) \mathrm{Re}\, x_1 - 2 w_x c_1 c_4 - \lambda c_2^2}{\lambda c_2} \tag{141}$$

$$\mathrm{Im}\, y_2 = \frac{\lambda c_4 \mathrm{Re}\, x_1 + 2 w_y c_2 c_6 + \lambda c_4^2}{2 c_2 w_y (c_4^2 + c_6^2)}\,. \tag{142}$$

Let's first consider case B. Substituting $\lambda = \pm\lambda_0$ into the two equations above, we get from Eq.(141)

$$\mathrm{Im}\, y_2 = \pm \frac{c_4 \sqrt{w_x} \sqrt{c_1^2 + c_2^2}}{\sqrt{w_y} \sqrt{c_4^2 + c_6^2}} \mathrm{Re}\, x_1 \mp \frac{2 w_x c_1 c_4}{\lambda_0 c_2} - c_2 \tag{143}$$

and from Eq.(142)

$$\mathrm{Im}\, y_2 = \pm \frac{c_4 \sqrt{w_x} \sqrt{c_1^2 + c_2^2}}{\sqrt{w_y} \sqrt{c_4^2 + c_6^2}} \mathrm{Re}\, x_1 + \frac{2 w_y c_2 c_6 \pm \lambda_0 c_4^2}{2 c_2 w_y (c_4^2 + c_6^2)}\,. \tag{144}$$

Except in the special case where

$$\mp \frac{2 w_x c_1 c_4}{\lambda_0 c_2} - c_2 = \frac{2 w_y c_2 c_6 \pm \lambda_0 c_4^2}{2 c_2 w_y (c_4^2 + c_6^2)}\,, \tag{145}$$

case B will not have a solution.

Next we consider case A. Now the constraint (134) becomes

$$\mathrm{Re}\, x_1 \mathrm{Im}\, y_2 + c_2 \mathrm{Re}\, x_1 + c_4 \mathrm{Im}\, y_2 = 0\ . \tag{146}$$

The remaining task is to solve for $\mathrm{Re}\, x_1$, $\mathrm{Im}\, y_2$ and $\lambda$ from Eqns. (141), (142) and (146). The solution to this is given by

$$\lambda = \frac{2w_x c_4(c_1^2+c_2^2)\mathrm{Re}\, x_1 - 2w_x c_1 c_4}{c_2^2 + c_2 \mathrm{Im}\, y_2} \tag{147}$$

$$\mathrm{Re}\, x_1 = -\frac{c_4 \mathrm{Im}\, y_2}{c_2 + \mathrm{Im}\, y_2} \tag{148}$$

$$\tag{149}$$

and $\mathrm{Im}\, y_2$ is given by the solution to

$$-w_x c_4(c_1^2+c_2^2)\left(\frac{c_4}{c_2+\mathrm{Im}\, y_2}\right)^3 \mathrm{Im}\, y_2 - w_x c_1 c_4 \left(\frac{c_4}{c_2+\mathrm{Im}\, y_2}\right)^2 = w_y c_2(c_4^2+c_6^2)\mathrm{Im}\, y_2 - w_y c_2 c_6\ . \tag{150}$$

When $w_x = 0$, we have

$$\mathrm{Im}\, y_2 = \frac{c_6}{c_4^2+c_6^2} \tag{151}$$

$$= -\frac{\sqrt{t\, v_{2x}}}{t\, v_{2x} - t\, v_{1x} + v_{1x}} =: (\mathrm{Im}\, y_2)_{\max}\ . \tag{152}$$

When $w_y = 0$, we have

$$\mathrm{Im}\, y_2 = -\frac{c_1 c_2}{c_1 + c_4(c_1^2+c_2^2)} \tag{153}$$

$$= -\frac{\sqrt{t\, v_{2x}}}{t\, v_{2x} - t\, v_{1x}} =: (\mathrm{Im}\, y_2)_{\min}\ . \tag{154}$$

The Holevo-CR bound becomes

$$w_x v_x + w_y v_y \geq f_{\mathrm{HCR}} = w_x \underbrace{\frac{c_4^2(\mathrm{Im}\, y_2)^2 + (1-c_6\mathrm{Im}\, y_2)^2}{(c_2+\mathrm{Im}\, y_2)^2}}_{f_x} + w_y \underbrace{\frac{c_4^2(\mathrm{Im}\, y_2)^2 + (1-c_6\mathrm{Im}\, y_2)^2}{c_4^2}}_{f_y}\ , \tag{155}$$

where $(\mathrm{Im}\, y_2)_{\min} \leq \mathrm{Im}\, y_2 \leq (\mathrm{Im}\, y_2)_{\max}$ is obtained by solving (150). Each value of $w_x/w_y$ defines a straight line in the $(v_x, v_y)$ plane. Several of these lines are plotted in Fig. 4. The envelope of these lines as we vary $w_x/w_y$ defines the curve parametrised by $v_x = f_x(\mathrm{Im}\, y_2)$ and $v_y = f_y(\mathrm{Im}\, y_2)$.

#### *4. Step 4: Optimising the splitting ratio t*

Next, we want to find the accessible variances as we change the splitting ratio $t$. Each value of $t$ parametrises a curve given by

$$v_x = f_x(\mathrm{Im}\, y_2, t) = \frac{(1-t)v_{1x}(\mathrm{Im}\, y_2)^2 + (1+\sqrt{t\, v_{2x}}\mathrm{Im}\, y_2)^2}{(\sqrt{t\, v_{2y}} + \mathrm{Im}\, y_2)^2} \tag{156}$$

$$v_y = f_y(\mathrm{Im}\, y_2, t) = \frac{(1-t)v_{1x}(\mathrm{Im}\, y_2)^2 + (1+\sqrt{t\, v_{2x}}\mathrm{Im}\, y_2)^2}{(1-t)v_{1x}}\ . \tag{157}$$

Several of these curves are plotted in Fig. 5. The envelope of all these curves can be obtained by solving

$$\frac{\partial f_x}{\partial t}\frac{\partial f_y}{\partial \mathrm{Im}\, y_2} = \frac{\partial f_x}{\partial \mathrm{Im}\, y_2}\frac{\partial f_y}{\partial t}\ . \tag{158}$$

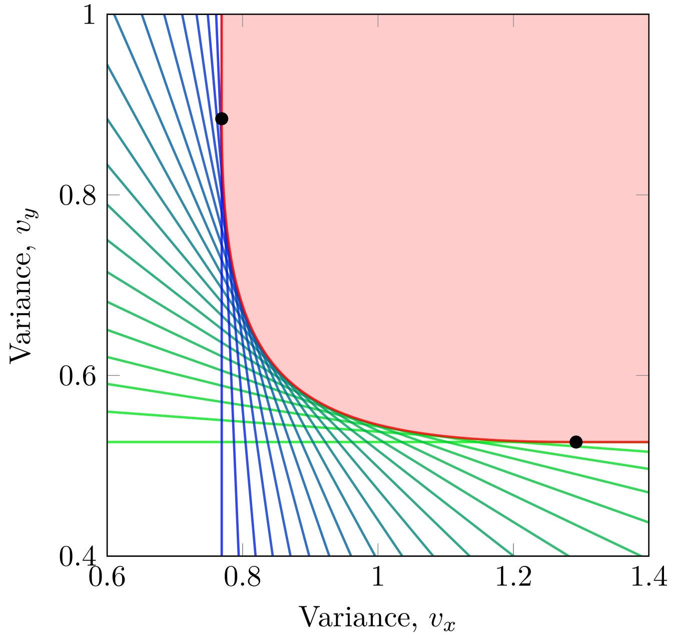


FIG. 4. Each of the straight line is given by Eqn. (155) and parametrised by a value of $w_x/w_y$. The red curve is the envelope of all these lines and can be parametrised by $v_x = f_x(\operatorname{Im} y_2)$ and $v_y = f_y(\operatorname{Im} y_2)$. At the two black dots, we have $\operatorname{Im} y_2 = (\operatorname{Im} y_2)_{\min}$ and $\operatorname{Im} y_2 = (\operatorname{Im} y_2)_{\max}$. In this plot, we have $r_1 = 0.35$, $r_2 = 0.69$, $t = 0.4$, $\phi_1 = 0$ and $\phi_2 = \pi/2$.

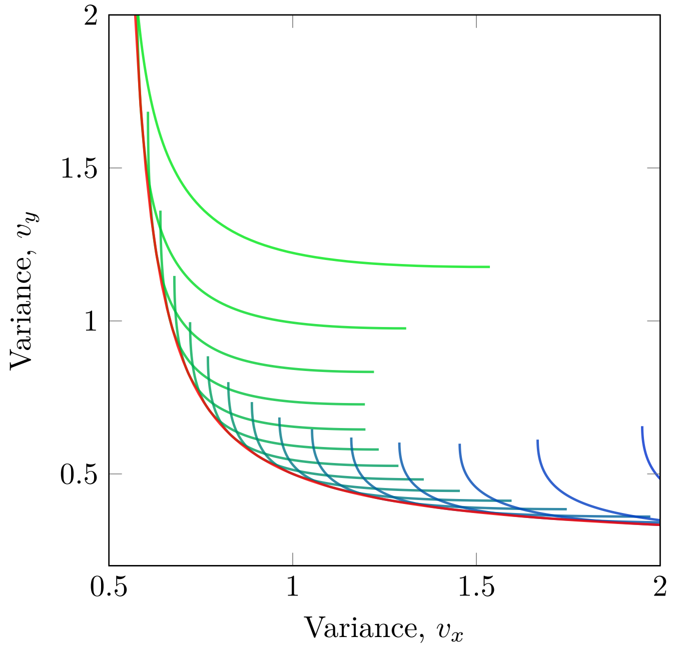


FIG. 5. Each of the bluish-green curve is the accessible region for a fixed $t$ parametrised by Eqns. (156) and (157). The red curve is the envelope of all these and given by Eqn. (161). In this plot, we have $r_1 = 0.35$, $r_2 = 0.69$, $\phi_1 = 0$ and $\phi_2 = \pi/2$.

The solution to this is given by

$$\operatorname{Im} y_2 = -\sqrt{\frac{v_{2y}}{t}} \,. \tag{159}$$

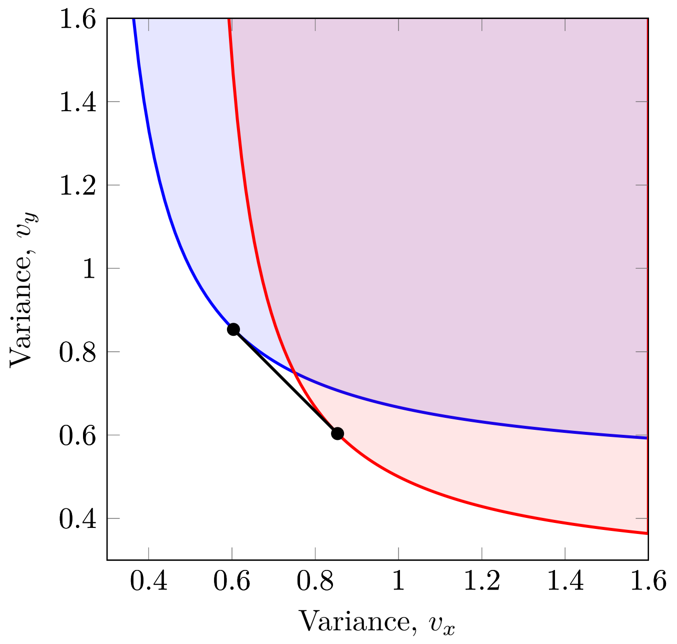


FIG. 6. The red and blue curves show the bounds from Eqs. (162) and (163) where ($\phi_1 = 0$, $\phi_2 = \pi/2$) and ($\phi_1 = \pi/2$, $\phi_2 = 0$) respectively. The black straight line joining them can be accessed by varying $\phi_1$ whilst keeping $\phi_2 = \phi_1 + \pi/2$. In this plot, we have $r_1 = 0.35$, $r_2 = 0.69$.

Substituting this into Eqs. (156) and (157) gives

$$f_x(t) = \frac{v_{1x}}{1-t} \ , \ f_y(t) = \frac{v_{2y}}{t} \tag{160}$$

which can also be written as

$$\frac{v_{1x}}{v_x} + \frac{v_{2y}}{v_y} = 1 \ . \tag{161}$$

When $\phi_1 = 0$ and $\phi_2 = \pi/2$, this becomes

$$\frac{e^{-2r_1}}{v_x} + \frac{e^{-2r_2}}{v_y} = 1 \tag{162}$$

and when $\phi_1 = \pi/2$ and $\phi_2 = 0$, this becomes

$$\frac{e^{-2r_2}}{v_x} + \frac{e^{-2r_1}}{v_y} = 1 \ . \tag{163}$$

These two bounds are plotted in Fig. 6. When $w_x = w_y$, both values of $\phi_1 = 0$ and $\phi_1 = \pi/2$ perform equally well. In this case, as we have seen in Fig. 3, any value of $\phi_2 = \phi_1 + \pi/2$ will give the same $f_{\mathrm{HCR}}$. These allow us to access the regions in between the two bounds (162) and (163).

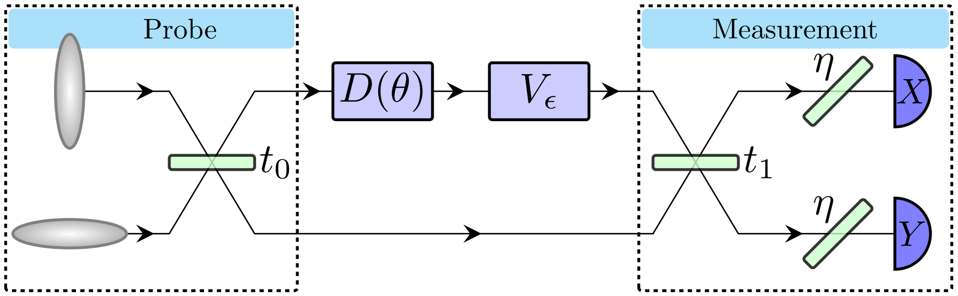


FIG. 7. We model the added noise in the channel by a random gaussian modulation with amplitude $V_\epsilon$ in both quadratures. Inefficient detectors are modelled by inserting a beam-splitter with transmissivity $\eta$. In the ideal setup with $V_\epsilon = 0$ and $\eta = 1$, the optimal measurement consist of interfering the two beams on a beam-splitter with transmissivity $t_1$ that depends on $t_0$, squeezing level $r$, and weighting ratios $w_x$ and $w_y$.

## IV. EFFECT OF CHANNEL NOISE AND LOSSY DETECTORS

In this section, we consider the effects of channel noise and lossy detectors for the two-mode probe example presented in the main text. The channel noise is modelled by adding a random Gaussian noise with variance $V_\epsilon$ in both quadratures. The lossy detectors are modelled by adding a beam-splitter with transmissivity $\eta$ before every detector.

We first consider the case where the first beam-splitter used to mix the probe has a fixed transmissivity $t_0 = 0.5$. The optimal measurement that minimises the Holevo-CR bound for a given $w_x/w_y$ is shown in Fig. 7 where the transmissivity of the beam-splitter $t_1$ depends on the ratio of the weights $w_x/w_y$. It is straightforward to show that the estimation variances with added noise $V_\epsilon$ and detector transmissivities $\eta$ are given by the pair $(v_x^*, v_y^*)$ where

$$v_x^* = \frac{\eta\left(\cosh 2r - 2\sqrt{t_1(1-t_1)}\sinh 2r + (1-t_1)V_\epsilon\right) + 1 - \eta}{\eta\,(1-t_1)}\,, \tag{164}$$

$$v_y^* = \frac{\eta\left(\cosh 2r - 2\sqrt{t_1(1-t_1)}\sinh 2r + t_1 V_\epsilon\right) + 1 - \eta}{\eta\,t_1}\,. \tag{165}$$

The accessible variances for some values of $V_\epsilon$ and $\eta$ are shown as the red shaded region in Fig. 8.

As mentioned in the main text, for the given weights $w_x$ and $w_y$, the optimal probe is formed by setting $t_0 = \frac{\sqrt{w_y}}{\sqrt{w_x}+\sqrt{w_y}}$. The optimal measurement is to set $t_1 = t_0$ in Fig. 7. It is once again straightforward to show that the estimation variances with added noise $V_\epsilon$ and detector transmissivities $\eta$ are given by the pair $(v_x^*, v_y^*)$ where

$$v_x^* = \frac{\eta\left(e^{-2r} + (1-t_0)V_\epsilon\right) + 1 - \eta}{\eta\,(1-t_0)}\,, \tag{166}$$

$$v_y^* = \frac{\eta\left(e^{-2r} + t_0 V_\epsilon\right) + 1 - \eta}{\eta\,t_0}\,. \tag{167}$$

The accessible variances for some values of $V_\epsilon$ and $\eta$ are shown as the grey shaded region in Fig. 8.

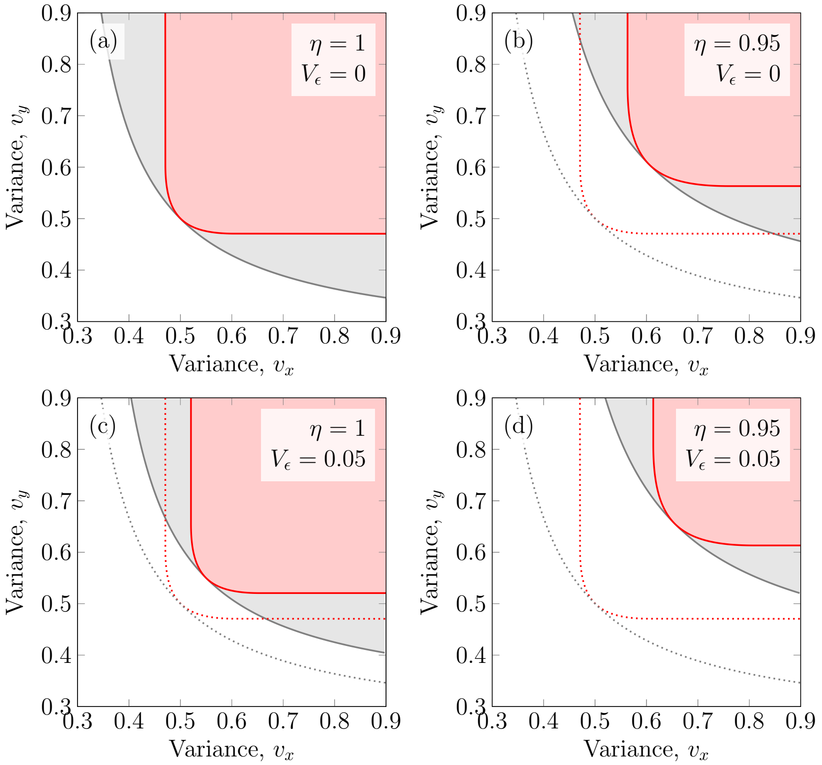


FIG. 8. (a) The accessible regions with two 6 dB squeezed resource ($r = 0.69$) assuming an ideal channel and perfect detectors are shown. The red line is the boundary for the probe with $t_0 = 0.5$ and where the optimal measurement is obtained by varying $t_1$. The grey line plots the performance of the optimal probe where $t_0 = t_1 = \frac{\sqrt{w_y}}{\sqrt{w_x}+\sqrt{w_y}}$. In (b), we simulate the effect of lossy detectors with $\eta = 0.95$ which shrinks the accessible region. In (c), we simulate the effect of added noise with $V_\epsilon = 0.05$—five percent of the vacuum fluctuations. Finally in (d), we consider both channel noise $V_\epsilon = 0.05$ and inefficient detectors $\eta = 0.95$. For comparison, the dotted lines in (b), (c) and (d) are the boundaries for the perfect channel.
